# Supplementary material for: Funnel-Transformer: Filtering out Sequential Redundancy for Efficient Language Processing
Source: arXiv:2006.03236 source file (2020-06-05)
Supplement: Supplementary file 1 [file appendix_back.tex]

\clearpage
\appendix
\section{Implementation Optimization}
\subsection{Sequence Truncation for Separating \cls Trick}
\label{sec:appendix-seq-trunc}

In the \name architecture, we introduce maintaining an independent \cls token during the pooling process.
It could lead to unexpected deceleration of the model speed. 
Assume that sequence length of an input sample is $2^p$, which usually is 512 in the pretraining phase. 
After one step pooling operation with the independent \cls token described in Section \ref{sec:proposed}, the length of the pooled sequence becomes $2^{p-1} + 1$, which makes the vector size does not align with an integer power of 2. 
Although one addition token would not cause substantive increasing in theoretical complexity, the model speed has the more obvious slowdown, roughly 10\% in GPU and 12\% in TPU, due to the hardware design of parallel computing device, which automatically pads the input vector to fit the size of parallel processors.  

To alleviate this issue, we propose to truncate the last token after pooling process when using the independent \cls. Denote the pooled hidden state as $\rvh = \{h_{cls}, h_0, \cdots,  h_{T-1}\}$, we truncate it by dropping last token,
\begin{equation}
\hat{\rvh} = \text{truncate}(\rvh) = \{h_{cls}, h_0, \cdots,  h_{T-2}\}
\end{equation}
Then, when the length of input sequence is a integer power of 2,  the length of the pooled sequence will keep as it. By applying this trick, the maintaining an independent \cls token design would not cause model slowdown. 

\subsection{Relative Positional Attention Implementation}
In this work, we use the relative positional attention parameterization proposed in the Transformer-XL~\cite{}.
To facilitate further discussion, we first review the details of this parameterization.
Taking the case of single head attention as the example head. 
Let $T, D$ be the sequence length and hidden dimension respectively.
Then, the pre-softmax attention score $A_{ij}$ between a pair of positions $i$ and $j$ consists of two terms:
\begin{align}
\label{eqn:rel_attn}
A_{ij} &= 
	\underbrace{ (W_Q h_i + v)^\top (W_K h_j) }_\text{ content term } + \underbrace{ (W_Q h_i + u)^\top (W_R r_{i-j}) }_\text{ position term }.
\end{align}
where $v, u \in \R^{D}$ are two trainable bias vectors, $W_Q, W_K, W_R \in \R^{D \times D}$ are three trainable projection matrices, and $r_{i-j} \in \R^{D}$ is the sinusoidal positional encoding that represents the relative distance $i-j$ between the two positions.

To compute the entire attention score matrix $\mb{A}$, the content term can easily be obtained via two head projections and an \textit{outer product} of complexity $O(TD^2 + T^2D)$:
\[ 
	\mb{A}^\text{content} = (\mb{H}W_Q + v) (\mb{H}W_K)^\top,
\]
where $\mb{H} = \seq{h_1, \cdots, h_T} \in \R^{T \times D}$ collects all hidden states into a matrix.
However, we cannot compute the position term in the same way as each $A_{ij}^\text{position}$ corresponds to a different $r_{i-j}$. 
Hence, a naive solution will be stacking $T^2$ pairs of position encodings into a tensor $\mb{\hat{R}} \in \R^{T\times T\times D}$ where $\mb{\hat{R}}_{ij} = r_{i-j}$, and then perform the following tensor product:
\[
	\mb{A}^\text{position} = \texttt{einsum}(\texttt{"id,ijd->ij"}, \mb{H}W_Q + u, \hat{\mb{R}}W_R).
\]
Note that the head projection $\mb{R}W_K$ now has a complexity of $O(T^2D^2)$ and a memory footprint of $O(T^2D)$, dominating all other computations.

\subsubsection{Standard Solution: Gather / Shift}
To resolve the computation burden above, a common technique is to instead collect a matrix $\mb{R} \in \R^{2T-1 \times D}$, where 
\[ \mb{R} = \seq{r_{T-1}, \dots, r_{0}, \cdots, r_{1-T}} \]
which includes all possible position encodings arranged from the maximum possible distance value $T-1$ to the minimum one $1 - T$.
Note that the full $\mb{\hat{R}}$ can be formed by gathering specific elements from $\mb{R}$ with an index matrix $\mb{I}$ of shape $[T \times T]$, i.e., 
\[ \mb{\hat{R}} = \text{gather}(\mb{R}, \mb{I}), \quad I_{ij} = T + i - j. \]
Mathematically, this is equivalent to using a permutation tensor $\mb{P} \in \R^{T \times T \times 2T-1}$ to multiply $\mb{R}$, i.e., $\mb{\hat{R}} = \mb{P} \mb{R}$, where $\mb{P}_{ij} \in \R^{2T-1}$ is a one-hot vector used to select/gather a single position of $\mb{R}$.
As the attention score computation only involves linear operations, we can rearrange the computation of the position term as follows
\begin{align*}
\mb{A}^\text{position} 
&= \texttt{einsum}\rbr{ \texttt{"id,ijd->ij"}, \mb{H}W_Q + u, \green{(\mb{P}\mb{R})} W_R } \\
&= \texttt{einsum}\rbr[\Big]{ \texttt{"ijk,jk->ij"}, \green{\mb{P}}, \sbr{ (\mb{H}W_Q + v) (\mb{R}W_R)^\top } } \\
&= \texttt{gather}\rbr[\Big]{ (\mb{H}W_Q + v) (\mb{R}W_R)^\top, \mb{I} }
\end{align*}
Note that, assuming gathering $T^2$ elements only has a complexity of $O(T^2)$, which is true for CPU/GPU, this trick reduces the computation complexity back to $O(2TD^2 + 2T^2D)$.
In practice, the gather operation can be implemented via a smart reshape operation, that is even cheaper.

\subsubsection{Optimization for TPU: factorized relative positional attention}
However, on TPUs, the assumption that gathering $T^2$ elements only has a complexity of $O(T^2)$ does not hold. 
Instead, we found that such a gather operation is dramatically slower on TPU.
Hence, we here consider another implementation which is significantly faster on TPU.

Firstly, let's rewrite the position term as follows
\begin{align}
A^\text{position}_{ij} 
&=  (W_Q h_i + u)^\top (W_R r_{i-j}) \nonumber\\
&=  \sbr[\Big]{\; \underbrace{ W_R^\top \rbr{ W_Q h_i + u}  }_{q_i} \;}^\top r_{i-j} \nonumber\\
\label{eqn:factorized-0}
&= q_i^\top r_{i-j}.
\end{align}
For easier derivation, we have introduced a notation of $q_i$. 
Then, recall the $r_{i-j}$ is the sinusoidal encoding that consists of the sine and the cosine components $r_{i-j} = \texttt{cat}(\sin_{i-j}, \cos_{i-j})$, where
\begin{align*}
\sin_{t} &= \seq{ \sin\rbr{t / 10000^{2/D}}, \sin\rbr{t / 10000^{4/D}}, \cdots, \sin\rbr{t / 10000^{D/D}} } \in \R^{D/2}, \\
\cos_{t} &= \seq{ \cos\rbr{t / 10000^{2/D}}, \cos\rbr{t / 10000^{4/D}}, \cdots, \cos\rbr{t / 10000^{D/D}} } \in \R^{D/2}.
\end{align*}
Hence, we similarly divide $q_i$ defined above into two parts, i.e., 
\[ q_i = \texttt{cat}(q_i^{\sin}, q_i^{\cos}). \]

Given the definitions, we can further break Eqn. \eqref{eqn:factorized-0} into two terms:
\begin{align*}
A^\text{position}_{ij} &= q_i^\top r_{i-j} = {q_i^{\sin}}^\top \sin_{i-j} + {q_i^{\cos}}^\top \cos_{i-j}.
\end{align*}
Now, using the trigonometric identities $\sin(a - b) = \sin(a)\cos(b) - \cos(a)\sin(b)$ and $\cos(a - b) = \cos(a)\cos(b) + \sin(a)\sin(b)$, the two terms can be respectively reformulated into
\begin{align*}
{q_i^{\sin}}^\top \sin_{i-j} 
&= {q_i^{\sin}}^\top \sbr{\sin_{i} \odot \cos_{j} - \cos_{i} \odot \sin_{j}} \\
&= {q_i^{\sin}}^\top \rbr{\sin_{i} \odot \cos_{j}} - {q_i^{\sin}}^\top \rbr{\cos_{i} \odot \sin_{j}} \\
&= \sbr{ q_i^{\sin} \odot \sin_{i} }^\top \cos_{j} + \sbr{ q_i^{\sin} \odot (-\cos_{i}) }^\top \sin_{j} \\
\intertext{and}
{q_i^{\cos}}^\top \cos_{i-j} 
&= {q_i^{\cos}}^\top \sbr{\cos_{i} \odot \cos_{j} + \sin_{i} \odot \sin_{j}} \\
&= {q_i^{\cos}}^\top \rbr{\cos_{i} \odot \cos_{j}} + {q_i^{\cos}}^\top \rbr{\sin_{i} \odot \sin_{j}} \\
&= \sbr{ q_i^{\cos} \odot \cos_{i} }^\top \cos_{j} + \sbr{ q_i^{\cos} \odot \sin_{i} }^\top \sin_{j}
\end{align*}

Hence, combining these two parts together, it follows that
\begin{align*}
q_i^\top r_{i-j} 
&= {q_i^{\sin}}^\top \sin_{i-j} + {q_i^{\cos}}^\top \cos_{i-j} \\
&= \sbr{ q_i^{\sin} \odot \sin_{i} }^\top \cos_{j} 
+ \sbr{ q_i^{\sin} \odot (-\cos_{i}) }^\top \sin_{j} 
+ \sbr{ q_i^{\cos} \odot \cos_{i} }^\top \cos_{j} 
+ \sbr{ q_i^{\cos} \odot \sin_{i} }^\top \sin_{j} \\
&= \cbr{ 
	\sbr{ q_i^{\sin} \odot \sin_{i} }^\top \cos_{j} + 
	\sbr{ q_i^{\cos} \odot \cos_{i} }^\top \cos_{j} } 
+ \cbr{
	\sbr{ q_i^{\sin} \odot (-\cos_{i}) }^\top \sin_{j} +
	\sbr{ q_i^{\cos} \odot \sin_{i} }^\top \sin_{j} } \\
&= \sbr[\bigg]{ 
		\underbrace{ \texttt{cat}( q_i^{\sin}, q_i^{\cos} ) }_{= q_i} \odot 
		\underbrace{ \texttt{cat}(\sin_{i}, \cos_{i}) }_{\coloneqq \phi_i} 
	}^\top \underbrace{ \texttt{cat}(\cos_{j}, \cos_{j} ) }_{\coloneqq \psi_j}\\ &\quad + 
   \sbr[\bigg]{ 
   		\underbrace{ \texttt{cat}(q_i^{\sin}, q_i^{\cos}) }_{= q_i} \odot 
   		\underbrace{ \texttt{cat}(-\cos_{i}, \sin_{i}) }_{\coloneqq \pi_i} 
   	}^\top \underbrace{ \texttt{cat}(\sin_{j}, \sin_{j})  }_{\coloneqq \omega_j} \\
&= \sbr{q_i \odot \phi_i }^\top \psi_j + \sbr{q_i \odot \pi_i}^\top \omega_j,
\end{align*}
where $\phi_i, \psi_j, \pi_i, \omega_j$ above are simply 4 positional encodings formed by concatenating the cosine and sine vectors of the corresponding $i$ and $j$ in different ways.
Note that, each term of the last line has a \textit{factorized} form that can be computed via an \textit{outer product}, just like the standard content term.
Therefore, by stacking $\phi_i, \psi_j, \pi_i, \omega_j$ of all positions (i.e. $i=1,\dots,T$ and $j=1,\dots,T$) into the corresponding $\mb{\Phi}, \mb{\Psi}, \mb{\Pi}, \mb{\Omega} \in \R^{T \times D}$ respectively, the full position term can be expressed in a simple form
\begin{align*}
\mb{A}^\text{position} 
&= \cbr[\Big]{ \sbr[\big]{ \rbr{ \mb{H} W_Q + u} W_R^\top } \odot \mb{\Phi}  } \mb{\Psi}^\top 
+ \cbr[\Big]{ \sbr[\big]{ \rbr{ \mb{H} W_Q + u} W_R^\top } \odot \mb{\Pi}  } \mb{\Omega}^\top 
\end{align*}
which leads to the complexity of $O(2TD^2 + 4T^2D)$, which is comparable to the content term.

\subsection{Potential Model Extensions}

\section{Experiment Setting and Hyper-parameters}
\label{sec:appendix-hparam}

\subsection{Hyperparameters for Pretraining}

\input{table/hyp-pretrain.tex}

The hyperparameters used for pretraining \name are shown in Table \ref{tab:hp-pretrain}. In the all experiments, we only annotate the size of hidden state. The rest of model hyper-parameters can be computed based on it. For example, assume the size of hidden state is $h$. The size of embedding is $h$. The size of inner states of P-FFN layer is $4 \times h$. The number of attention head is $h // 64$. The attention heads is always $64$.

\subsection{Hyperparameters for Finetuning}
\input{table/hyp-finetune.tex}

The hyperparameters used for finetuning on various tasks are shown in Table \ref{tab:hp-finetune}. 
we grid search the learning rates from the set $\{1e-5, 2e-5, 3e-5\}$, and choose the best one according to the validation set. 
``Layer-wise decay'' means exponentially decaying the learning rates of individual layers in a top-down manner. For example, suppose the $24$-th layer uses a learning rate $l$, and the Layer-wise decay rate is $\alpha$, then the learning rate of layer $m$ is $l \alpha^{24 - m}$.

All the experiment results are the median result of running the finetuning process with 5 different random seeds. 

\section{Additional Experimental Results}
\label{sec:appendix-extra-exp}
\subsection{Ablation Study}
\label{sec:appendix-ablation}

\begin{table}[!ht]
	\resizebox{\textwidth}{!}{
		\begin{tabular}{@{}lcccc|c@{}}
			\toprule
			Layout (FLOPs/Params) & Pool-Op & Pool-query-only & Sep \cls  & TFM-XL        & GLUE-AVG  \\
			\midrule
			(1)B6-6-6 (1.00x / 1.00x)
			& Mean     & \checkmark & \checkmark & \checkmark & \textbf{83.5} \\
			(2)& Mean     & \checkmark &            & \checkmark & 82.9 \\
			(3)& Mean     &            & \checkmark & \checkmark & 83.1 \\
			(4)& Mean     & \checkmark & \checkmark &            & 81.4 \\
			(5)& Max      & \checkmark & \checkmark & \checkmark & 83.4 \\
			(6)& Top-Attn & \checkmark & \checkmark & \checkmark & 75.8 \\
			(7)B8-8  (1.14x / 0.91x)
			& Mean     & \checkmark & \checkmark & \checkmark & 83.4 \\
			(8)B5-5-5-5 (0.89x / 1.08x)
			& Mean     & \checkmark & \checkmark & \checkmark & 82.9 \\
			%(9)B6-3x2-3x2 (1.00x / 0.73x)
			%& Mean     & \checkmark & \checkmark & \checkmark & 82.8 \\
			\bottomrule
	\end{tabular}}
	\caption{Ablation Results}
	\label{tab:ablation}
\end{table}

In this section, we conduct an ablation study to verify the importance of following designs of F-TFM: 
\begin{itemize}[leftmargin=*]
	\item Choice of pooling operation: We test the proposed model with two-classes pooling operations:
	\begin{itemize}
		\item The first type is just the strided mean/max pooling described in section \ref{sec:method}
		\item The second type aims to select a subset of ``hub'' states, which refer to those hidden vectors that are attended most in the previous S-Attn layer and hence likely to carry most critical information about the sequence.
		Concretely, given the attention map from the previous S-Attn layer, we reduce sum the scores along the number of head and query length dimensions to a score for each position.
		Then, we simply choose the top 50\% of states to achieve the same compression rate.
	\end{itemize}
	\item Pool-query-only design
	\item Separating \cls in the pooling operation
	\item Relative position embedding proposed in TFM-XL \cite{}. We compare this operation with the learned absolute position embedding used in Bert model \cite{}.
	\item We compare the 3-blocks design with 2-blocks and 4-blocks design. 
\end{itemize}

The ablation results are included in table \ref{tab:ablation}. The size of model hidden states in table \ref{tab:ablation} is 512. We have following observations:

\begin{itemize}[leftmargin=*]
	\item Comparing different operation ((1), (5) and (6)), we found that the performance of mean and max pooling operation is similar. But they are significant better than the idea of utilizing attention score (Top-Attn pooling) to select the ``hub'' states, which means that the spatial prior is better under the current architecture and optimization technique. 
	\item Comparing (1) and (3), we see that the pool-query-only design could bring the noticeable improvement to the proposed model. Comparing (1) and (2), we found that the Sep \cls trick also provides similar improvement. 
	\item Comparing (1) and (4), it shows that the relative position embedding introduced in TFM-XL provides the significant improvement on the final results. It is necessary to the proposed model.
	\item Comparing (1), (7) and (8), we found that the 3-blocks design is the best one to achieve the balance between flops and performance. In order to better compare them, we make the size of their parameter as similar as possible.  
\end{itemize}

\subsection{Training Cost Comparison}
\label{sec:appendix-training-cost}
\input{table/gpu-time.tex}
\input{table/tpu-time.tex}
\input{table/pretrain-time.tex}

In table \ref{tab:gpu-time} and \ref{tab:tpu-time}, we compare the finetuning speed of the models on a 8-GPUs (V100) system and a 8-cores TPU-v2 system. 
In the GPU experiment, we use Pytorch and ``O2'' options of AMP manager in the apex package to handle the FP16 optimization. 
In the TPU experiment, we use the TensorFlow package with the FP16 optimizer. For each case, we choose the largest possible batch size according to the memory size of the devices. 

From experiment results, we observe that the speed of B6\_6\_6H768 is similar or faster than the Bert-Base model, while B6\_6\_6H768 is deeper, has more parameters, and can achieve better results compared with Bert-Base model.
This conclusion can be applied to the B6\_3x2\_3x2H768 and B4\_4x2\_4x2H768  models. The B4\_4\_4H768 model, which has the same depth and model parameters as the Bert-Base model, is able to provide 30\%-50\% speedup without losing too much performance. 
In the Bert-Large based comparison, the conclusion is similar. The speed of the larger model B10\_10\_10H768 is almost the same as the Bert-Large model, and the speed of B8\_8\_8H768 is significantly faster than Bert-Large model.

In the above part, we majorly discuss the model speed in the finetuning stage. 
It does not required the decoder component, which is designed for the masked language model training in the pretraining stage (described in section \ref{sec:method}).
So, to fairly compare the model efficiency in the pretraining stage, we include the model training speed with the decoder component in table \ref{tab:tpu-pre-time}. 
The results show that the proposed method can also improve the pretraining speed compared with the vanilla Bert architecture, although the improved percentage is slightly smaller than the finetuning stage.  
In summary, this study demonstrates that the proposed method is more efficient in both the finetuning and pretraining stages.
